# Supplementary material for: GraphX-Convolution for Point Cloud Deformation in 2D-to-3D Conversion
Source: arXiv:1911.06600 ancillary file (2019-11-15)
Supplement: Supplementary file 1 [file graphx-conv-supp.pdf]

# GraphX-Convolution for Point Cloud Deformation in 2D-to-3D Conversion (Supplementary)

Anh-Duc Nguyen Seonghwa Choi Woojae Kim Sanghoon Lee
Yonsei University
{adnguyen,csh0772,wooyoa,slee}@yonsei.ac.kr

## 1. Relation to Graph Convoluton

We consider Graph Convoluton without the bias term as follows

$$y_i = W_1 x_i + \sum_{x_k \in \mathcal{N}(x_i)} W_2^T x_k \tag{1}$$

where $W_1$ and $W_2$ are trainable, and $\mathcal{N}(x_i)$ is the set of nodes connecting to $x_i$. As pointed out in the main paper, to reduce computation, we first unify the two weights

$$\begin{aligned} y_i &= \sum_{x_k \in \mathcal{N}(x_i) \cup \{x_i\}} W^T x_k \\ &= W^T \sum_{x_k \in \mathcal{N}(x_i) \cup \{x_i\}} x_k \end{aligned}. \tag{2}$$

Our goal is to design an operator that conditions on the whole input set to make inference for each point, so we calculate the sum over the whole point cloud instead

$$y_i = W^T \sum_{x_k \in \mathcal{X}} x_k. \tag{3}$$

However, some points can be more important than others. To reflect this, we weight the importance of each point by a trainable factor

$$y_i = W^T \sum_{x_k \in \mathcal{X}} w_k x_k, \tag{4}$$

which is the bias-free version of GraphX.

## 2. Theoretical analysis of GraphX

In this section, we try to supplement some theoretical background on why we are sure GraphX would work in the first place. Let $p(C)$ denote the prior distribution of the category of an object; for *e.g.*, $C$ can be a chair or a bed. For each category, there is a wide variety of models; for instance, a chair can have wheels or legs. Thus, we use $p(M|C)$ to characterize a specific model given an item class. Finally, since there can be numerous point cloud feature representations of a model, let us define $p(P|M,C)$ to be the distribution of a point in a point cloud of a certain model in a fixed class. We can see that each random sample $(P_1, P_2, ..., P_n) \sim p(P|M,C)$ is a possible point cloud configuration of the given model. We note that a point cloud here does not restrict to the 3D representation but could be a cloud of feature vectors as well.

The mixing operation in GraphX takes a point cloud configuration and returns a new one. Let the mixing weights for a point $Y_j$ be $w_{jk}$. In mathematical expressions, the mixing can be written as

$$Y_j = \sum_k w_{jk} P_k. \tag{5}$$

For the sake of simplicity, we omit the bias. It then follows that

$$\begin{aligned} E[Y_j] &= E[\sum_k w_{jk} P_k] \\ &= E_{p(P|M,C)}[P] \sum_k E[w_{jk}] \\ &= n E_{p(P|M,C)}[P] E[w_j]. \end{aligned} \tag{6}$$

It can be seen that GraphX evaluates the mean of the point cloud distribution and then scales it. In our implementation, the original point cloud is drawn from a uniform distribution, and hence the mean can be estimated by the sample mean, which explains why the mixing weights learn to average and scale all the points as shown in Section 4.3. Certainly, learning the mean may just be the face value, as we have pointed out when averaging and scaling manually, the performance became much worse. Nonetheless, this viewpoint is interesting because the layer size can be truly independent from the input point cloud size, which enables the system to be more scalable. This will be covered in our upcoming research.

In other problems such as point cloud analysis, when the point cloud distribution is not trivial like in our case, the mixing weights can learn a more interesting distribution. We do not learn separate mixing coefficients but share

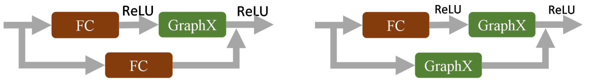


Figure 1. Residual GraphX blocks: (a) ResGraphX and (b) UpResGraphX.

them for different models and categories, so they can learn the joint model $p(P, M, C)$, not just $p(P|M, C)$ like in (6). In other words, the mixing matrix learns at a distribution level, which separates GraphX from the graph convolution or $\mathcal{X}$-conv which only learns at an instance level. However, because of the stacking of many layers, the theoretical viewpoint we share here is still very superficial and more technical details should be elaborated in order to grasp the true essence of GraphX.

# 3. Architecture details

The detailed configurations of the image encoding and point cloud encoding branches are described in Table 1. The image encoder is the same as in [5]. The point cloud encoder has the same number of blocks as the image encoder (4 in our implementation), and each block comprises of two FC layers of the same size. We have tried some other VGG architectures as well, such as VGG16 and VGG19 [4], but no improvement has been recorded.

There are some implementation details worth pointing out here. In the formulation of GraphX, we can apply an activation after the mixing and/or exchange the order of the mixing and fully connected layer. However, while the former does not have much of an impact on the overall result, the latter significantly reduces the performance. This is curiously surprising because except for the bias terms, the transformed feature is the same in both cases. Due to the aforementioned reasons, the definition of GraphX is finalized as in the paper.

The ResGraphX and UpResGraphX architectures are shown in Figure 1. In both configurations, the first layer of the main branch is an FC followed by a ReLU. The second layer is either a basic GraphX layer in ResGraphX or the upsampling version of GraphX in UpResGraphX. In the residual branch, the layer is either an identity, FC or GraphX depending on the output size and the type of the block. The ResFC layer has the same spirit as ResGraphX but with the GraphX layer replaced by an FC.

The architectures of the five variants of the deformation network used in the paper are tabulated in Table 2. In all cases except for the UpResGraphX network, the initial point cloud had 2k points. For the UpResGraphX case, we used only a point cloud of 250 points, and the cloud doubled the size after each UpResGraphX layer, which also outputs a 2k-point cloud as other versions.

# 4. Additional results

This section presents the qualitative results of the simplified UpResGraphX layer that we hypothesized in Section 4.3 of the paper. The results are displayed in Table 3. For better comparison, we also include the results of other methods in the paper. As can be seen from the table, even though the model still achieves high CD performance, the IoU score is the worst among all the competing methods. In order to make it a practical method, more effort should be invested to further improve on this baseline.

# References

[1] Christopher B Choy, Danfei Xu, JunYoung Gwak, Kevin Chen, and Silvio Savarese. 3D-R2N2: A unified approach for single and multi-view 3D object reconstruction. In *Proceedings of the European Conference on Computer Vision (ECCV)*, pages 628–644. Springer, 2016.

[2] Haoqiang Fan, Hao Su, and Leonidas J Guibas. A point set generation network for 3D object reconstruction from a single image. In *Proceedings of the IEEE conference on Computer Vision and Pattern Recognition (CVPR)*, pages 605–613, 2017.

[3] Li Jiang, Shaoshuai Shi, Xiaojuan Qi, and Jiaya Jia. GAL: Geometric adversarial loss for single-view 3D-object reconstruction. In *Proceedings of the European Conference on Computer Vision (ECCV)*, pages 802–816, 2018.

[4] Karen Simonyan and Andrew Zisserman. Very deep convolutional networks for large-scale image recognition. *arXiv preprint arXiv:1409.1556*, 2014.

[5] Nanyang Wang, Yinda Zhang, Zhuwen Li, Yanwei Fu, Wei Liu, and Yu-Gang Jiang. Pixel2mesh: Generating 3D mesh models from single rgb images. In *Proceedings of the European Conference on Computer Vision (ECCV)*, pages 52–67, 2018.

Table 1. Architecture details of the image encoding and point cloud encoding networks. <n> × <Name>-<k> stands for a stack of $n$ <Name> layers with $k$ output channels/features.

| | pre-block | block 1 | block 2 | block 3 | block 4 |
|---|---|---|---|---|---|
| image encoder | 2 x Conv3-16<br>2 x Conv3-32 | 2 x Conv3-64 | 2 x Conv3-128 | 2 x Conv3-256 | 2 x Conv3-512 |
| point cloud encoder | n/a | 2 x FC-64 | 2 x FC-128 | 2 x FC-256 | 2 x FC-512 |

Table 2. Detailed architectures of different variants of the deformation network.

| FC | ResFC | GraphX | ResGraphX | UpResGraphX |
|---|---|---|---|---|
| FC-512 | ResFC-512 | GraphX-2k-512 | ResGraphX-2k-512 | UpResGraphX-500-512 |
| FC-256 | ResFC-256 | GraphX-2k-256 | ResGraphX-2k-256 | UpResGraphX-1k-256 |
| FC-128 | ResFC-128 | GraphX-2k-128 | ResGraphX-2k-128 | UpResGraphX-2k-128 |
| FC-3 | FC-3 | FC-3 | FC-3 | FC-3 |

Table 3. Quantitative results of UpResGraphXSim and other benchmarking methods on 13 major categories of ShapeNet. "↑" indicates higher is better. "↓" specifies the opposition. Best performance is highlighted in **bold**.

| Category | | table | car | chair | plane | couch | firearm | lamp | watercraft | bench | speaker | cabinet | monitor | cellphone | mean |
|---|---|---|---|---|---|---|---|---|---|---|---|---|---|---|---|
| CD↓ | 3D-R2N2 [1] | 1.116 | 0.845 | 1.432 | 0.895 | 1.135 | 0.993 | 4.009 | 1.215 | 1.891 | 1.507 | 0.735 | 1.707 | 1.137 | 1.445 |
| | PSG [2] | 0.517 | 0.333 | 0.645 | 0.430 | 0.549 | 0.423 | 1.193 | 0.633 | 0.629 | 0.756 | 0.439 | 0.722 | 0.438 | 0.593 |
| | Pixel2mesh [5] | 0.498 | 0.268 | 0.610 | 0.477 | 0.490 | 0.453 | 1.295 | 0.670 | 0.624 | 0.739 | 0.381 | 0.755 | 0.421 | 0.591 |
| | Ours (UpResGraphXSim) | 0.383 | 0.237 | 0.406 | 0.165 | 0.322 | 0.153 | 0.606 | 0.242 | 0.269 | 0.461 | 0.307 | 0.301 | 0.189 | 0.311 |
| | Ours (UpResGraphX) | **0.284** | **0.184** | **0.306** | **0.116** | **0.254** | **0.119** | **0.523** | **0.210** | **0.189** | **0.419** | **0.265** | **0.248** | **0.155** | **0.252** |
| IoU↑ | 3D-R2N2 [1] | 0.580 | **0.836** | 0.550 | 0.561 | 0.706 | 0.600 | 0.421 | 0.610 | 0.527 | 0.717 | **0.772** | 0.565 | 0.754 | 0.631 |
| | PSG [2] | 0.606 | 0.831 | 0.544 | 0.601 | 0.708 | 0.604 | 0.462 | 0.611 | 0.550 | **0.737** | 0.771 | 0.552 | 0.749 | 0.640 |
| | GAL [3] | **0.714** | 0.737 | **0.700** | 0.685 | 0.739 | 0.715 | **0.670** | 0.675 | 0.709 | 0.698 | **0.772** | **0.804** | 0.773 | 0.712 |
| | Ours (UpResGraphXSim) | 0.363 | 0.590 | 0.416 | 0.668 | 0.510 | 0.660 | 0.429 | 0.605 | 0.482 | 0.455 | 0.485 | 0.559 | 0.658 | 0.529 |
| | Ours (UpResGraphX) | 0.605 | 0.819 | 0.663 | **0.758** | **0.770** | **0.747** | 0.516 | **0.754** | **0.725** | 0.708 | 0.770 | 0.735 | **0.857** | **0.725** |
